# Supplementary material for: The maximum penalty criterion for ridge regression: application to the calibration of the force constant in elastic network models
Source: arXiv:1512.08294 ancillary file (2015-12-28)
Supplement: Supplementary file 1 [file SuppMat.pdf]

# Supplementary Material for the paper: The maximum penalty criterion for ridge regression: application to the calibration of the force constant in elastic network models


Ugo Bastolla[(1)] and Yves Dehouck[(2)]

[(1)] Centro de Biologia Molecular "Severo Ochoa"

CSIC-UAM Cantoblanco, 28049 Madrid, Spain. E-mail: ubastolla@cbm.csic.es

[(2)] Machine Learning Group, Université Libre de Bruxelles (ULB).

Boulevard du Triomphe CP 212, 1050 Brussels, Belgium. E-mail: ydehouck@ulb.ac.be


## Supplementary Text


Alternative definitions of the Maximum Penalty (MP) fit . . . . . . . . . . . . . . 2


## Supplementary Figures


S1 Performances of the alternative definitions of MP . . . . . . . . . . . . . . . . 4

S2 Error of the fitted internal motions when $T = 0$ or $R = 0$ . . . . . . . . . . . 5

S3 Error on the logarithm of the estimated force constant . . . . . . . . . . . . 5

S4 Error on the estimated fractions of rigid-body fluctuations . . . . . . . . . . 6

S5 Standard deviation of the logarithm of the force constant versus the average ridge parameter . . . . . . . . . . . . . . . . . . . . . . . . . . . . . . 6

# Alternative definitions of the Maximum Penalty fit

In ridge regression, the objective function to be minimised can usually be written as:

$$G^{(\mathrm{ns})} = E + \Lambda\,(\mathbf{a}, \mathbf{a})\ , \tag{S1}$$

where $E$ is the error of the fit, $\Lambda$ is the ridge parameter, and $\mathbf{a}$ is the $P$-dimensional vector of the fit parameters. We introduced in this paper a more general definition of the ridge regression problem, by adding a second lagrange multiplier $\mu$, so that the constraint $H$ ensuring the correct scale of the fit parameters $\mathbf{a}$ is respected even if the intercept of the fit is penalised as any other variable (Eq. 4 in the main text). The objective function to be minimized in rescaled ridge regression can be formulated as:

$$G^{(\mathrm{sc})} = E + (1-\mu)\Lambda\,((\mathbf{a}-\mathbf{a}^{\circ}), (\mathbf{a}-\mathbf{a}^{\circ})) + \mu H\ , \tag{S2}$$

where $\mathbf{a}^{\circ}$ are reference values of the fit parameters. We showed that the values of the parameters $\mathbf{a}^{(\mathrm{sc})}$ that minimize the objective function $G^{(\mathrm{sc})}$ (rescaled ridge regression) are equal to the parameters $\mathbf{a}^{(\mathrm{ns})}$ minimizing the objective function $G^{(\mathrm{ns})}$ (non-scaled ridge regression), up to a scaling factor, at the condition that the reference parameters are chosen as

$$\mathbf{a}^{\circ} = \xi(\Lambda)\mathbf{X}^T\mathbf{y} = \xi \sum_{\alpha} y^{\alpha} u_k^{\alpha}, \tag{S3}$$

where $u^{\alpha}$ is the $\alpha$-th eigenvector of the covariance matrix of the explanatory variables, $\mathbf{X}^T\mathbf{X}$, with eigenvalue $\lambda_{\alpha}$, and $\xi(\Lambda)$ satisfies the equation

$$\frac{1-\mu/2}{1-\mu} + \Lambda\xi(\Lambda) = 1 + \Lambda\eta(\Lambda) \tag{S4}$$

$$\eta(\Lambda) \equiv \frac{\sum_{\alpha} \frac{(y^{\alpha})^2}{(\lambda_{\alpha}+\Lambda)^2}}{\sum_{\alpha} \lambda_{\alpha} \frac{(y^{\alpha})^2}{(\lambda_{\alpha}+\Lambda)^2}} \tag{S5}$$

We proposed a criterion for choosing the ridge parameter $\Lambda$ that is based on the "entropic" contribution to the free energy of the fit, or penalty term,

$$\mathrm{Penalty}(\Lambda) = (1-\mu)\Lambda\,((\mathbf{a}-\mathbf{a}^{\circ}), (\mathbf{a}-\mathbf{a}^{\circ}))\ . \tag{S6}$$

The penalty term is equal to zero both at $\Lambda = 0$, where all the information of the correlation between explanatory variables is retained, and for $\Lambda \to \infty$, where $\mathbf{a}$ and $\mathbf{a}^{\circ}$ reach the same limit and the information of the correlation matrix is lost (except for the scaling factor). In between, the penalty term reaches a maximum, and we hypothesize that this maximum corresponds to a possibly optimal choice of the ridge parameter $\Lambda$. We call "maximum penalty fit" ridge regression with this choice of $\Lambda$.

In non-scaled ridge regression (Eq. S1), $\mu$ and all reference parameters $\mathbf{a}^{\circ}$ are equal to 0. The definition of the MP fit is thus unequivocal, as the value of $\Lambda$ identified by the MP

criterion is the one that maximizes the penalty term, i.e. $\Lambda_{\text{MP}} = \max_\Lambda \left(\Lambda\left(\mathbf{a}^{(\text{ns})}, \mathbf{a}^{(\text{ns})}\right)\right)$. With the more general definition of rescaled ridge regression (Eq. S2), there is some flexibility in the definition of the penalty term, and thus of the MP criterion, depending on the choice of the reference parameters $\mathbf{a}^\circ$. In addition to the definition retained in the main text, we also tested three slightly different definitions of the MP criterion, which are presented below.

**MP criterion**. The criterion presented in the main text consists in choosing reference parameters independent of $\Lambda$, which requires that $\xi$ does not depend on $\Lambda$:

$$\text{MP}: \qquad \xi = \xi_\infty \equiv \lim_{\Lambda\to\infty} \eta(\Lambda) = \frac{\sum_\alpha (y^\alpha)^2}{\sum_\alpha (y^\alpha)^2 \lambda_\alpha}\,, \tag{S7}$$

$$\mu = \frac{2\Lambda\left(\eta(\Lambda) - \xi_\infty\right)}{1 + 2\Lambda\left(\eta(\Lambda) - \xi_\infty\right)}\,. \tag{S8}$$

In this way, the reference parameters are equal to the infinite $\Lambda$ limit of the fit parameters, i.e. $\mathbf{a}^\circ = \mathbf{a}_\infty \equiv \lim_{\Lambda\to\infty} \mathbf{a}^{(\text{sc})}$. Thus, $\Lambda_{\text{MP}} = \max_\Lambda \left((1-\mu)\Lambda(\mathbf{a}^{(\text{sc})} - \mathbf{a}_\infty, \mathbf{a}^{(\text{sc})} - \mathbf{a}_\infty)\right)$.

**MP* criterion**. A first variation is obtained as an approximation of the MP criterion, in which the reference parameters are identical, $\mathbf{a}^\circ = \mathbf{a}_\infty$, but the dependence of $\mu$ on $\Lambda$ is considered negligible in the range of interest of $\Lambda$ values. We have then, $\Lambda_{\text{MP}*} = \max_\Lambda \left(\Lambda(\mathbf{a}^{(\text{sc})} - \mathbf{a}_\infty, \mathbf{a}^{(\text{sc})} - \mathbf{a}_\infty)\right)$, which can be easier to implement than the MP criterion but gives highly similar results, as shown in Fig. S1.

**MP$_\Lambda$ criterion**. Another possibility is to set $\xi(\Lambda) = \eta(\Lambda)$, so that $\mu = 0$ (Eq. S4), and we do not have to explicitly impose the constraint on the scale of the parameters. The resulting criterion is defined by the equations

$$\text{MP}_\Lambda: \qquad \xi = \xi_\Lambda \equiv \eta(\Lambda) \equiv \frac{\sum_\alpha \frac{(y^\alpha)^2}{(\lambda_\alpha+\Lambda)^2}}{\sum_\alpha \lambda_\alpha \frac{(y^\alpha)^2}{(\lambda_\alpha+\Lambda)^2}}\,, \tag{S9}$$

$$\mu = 0\,. \tag{S10}$$

This particular choice of the reference parameters $\mathbf{a}^\circ = \mathbf{a}_\Lambda = \xi_\Lambda \mathbf{X}^T\mathbf{y}$ automatically ensures the optimal scaling of the $\mathbf{a}^{(\text{sc})}$. The objective function can thus be expressed as $G^{(\text{sc})} = E + \Lambda(\mathbf{a} - \mathbf{a}_\Lambda, \mathbf{a} - \mathbf{a}_\Lambda)$, without the need for an additional constraint on the scale (i.e. $\mu = 0$). The drawback is that $\xi$, and hence the reference parameters, depend on $\Lambda$. We found that the MP$_\Lambda$ criterion produces results that are generally similar, although slightly poorer on average, than those based on the above definition of MP with $\xi = \xi_\infty$.

**MP$_{\text{ns}}$ criterion**. The last alternative is obtained by setting $\xi = 0$, so that the reference parameters $\mathbf{a}^\circ$ are all equal to zero. In that case, the penalty term does not reach a maximum value in rescaled ridge regression, because $(\mathbf{a}^{(\text{sc})}, \mathbf{a}^{(\text{sc})})$ does not tend to zero

when $\Lambda \to \infty$. It does however reach a maximum value in non-scaled ridge regression. A possibility is thus to choose the parameter $\Lambda$ that maximizes the penalty in the non-scaled fit, $\Lambda_{\mathrm{MP_{ns}}} = \max_\Lambda \left(\Lambda(\mathbf{a}^{(\mathrm{ns})}, \mathbf{a}^{(\mathrm{ns})})\right)$, and apply it to the rescaled fit. In non-scaled ridge regression, $\mu = 0$, since we do not impose the optimal scale. We have thus

$$\mathrm{MP_{ns}}: \quad \xi = 0 \tag{S11}$$
$$\mu = 0\,. \tag{S12}$$

We found that this definition tends to select larger values of $\Lambda$, and thus to impose a stronger regularisation of the fit. It did yield particularly good results in some cases, but generally performs worse than the MP criterion with $\xi = \xi_\infty$.

# Supplementary figures

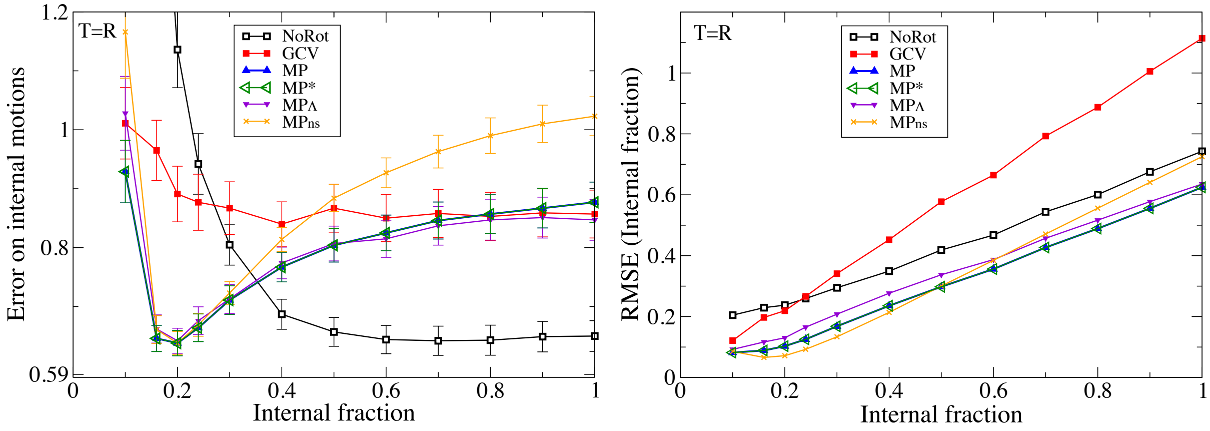


**Supplementary Figure S1: Performances of the alternative definitions of MP.** The error on the estimated profile of internal fluctuations (left), and the error on the estimated fraction of internal fluctuations (right) are given against the simulated fraction of internal fluctuations, $I$.

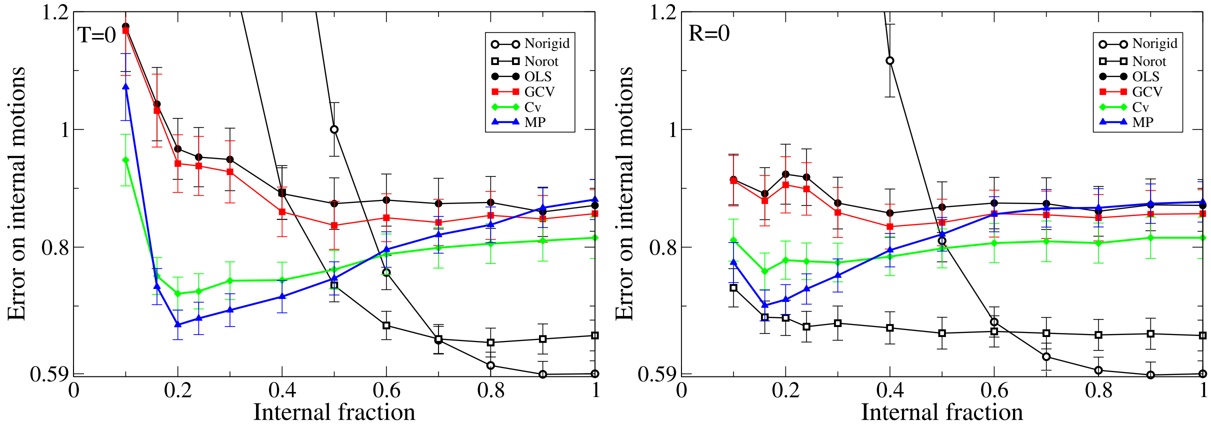


**Supplementary Figure S2: Error of the fitted internal motions when $T = 0$ or $R = 0$.** $E^{\text{int}}$ (see Eq. 22 in the main text) is given as a function of the fraction of internal motions $I$, in the simulated sets with either $T = 0$ (left) or $R = 0$ (right), for different types of fit. The lowest possible value of the error, $E^{\text{int}} = 0.59$, is obtained with the NoRigid fit on the NMR dataset ($I = 1.0$). One can see that for the $T = 0$ set with no translations the NoRot and NoRigid fits behave rather similarly.

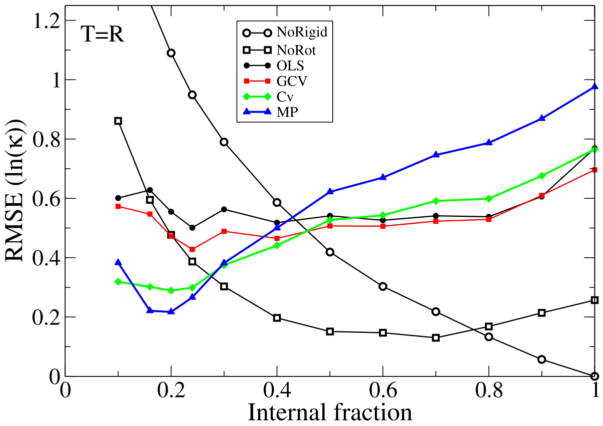


**Supplementary Figure S3: Error on the logarithm of the estimated force constant.** The RMSE of $\ln(\kappa)$ is given as a function of the internal fraction $I$, in the simulated sets with $T = R$. For $I \approx 0.2$, the MP fit is the best performer, as we also observed for the fitted fraction of internal motions (Fig. 3 in the main text).

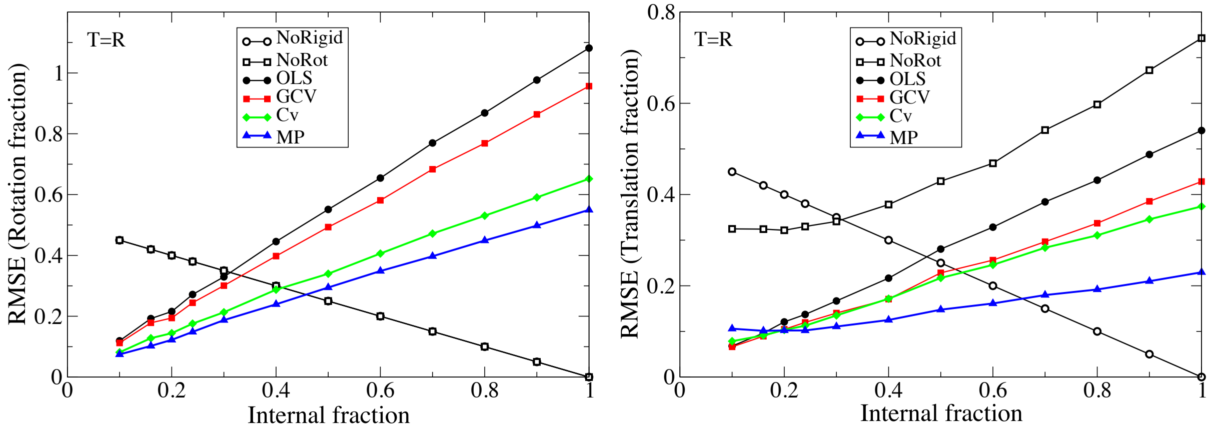


**Supplementary Figure S4: Error on the estimated fractions of rigid-body fluctuations.** The RMSE of the fitted rotational (left) and translational fractions (right) is given as a function of the internal fraction $I$. The error on the rotational fraction is the same for the NoRot and NoRigid fits, since the estimated fraction of motion due to rotations is always null in both fits. The MP fit is the best of all variants of ridge regression except for the translation fraction at $I < 0.2$.

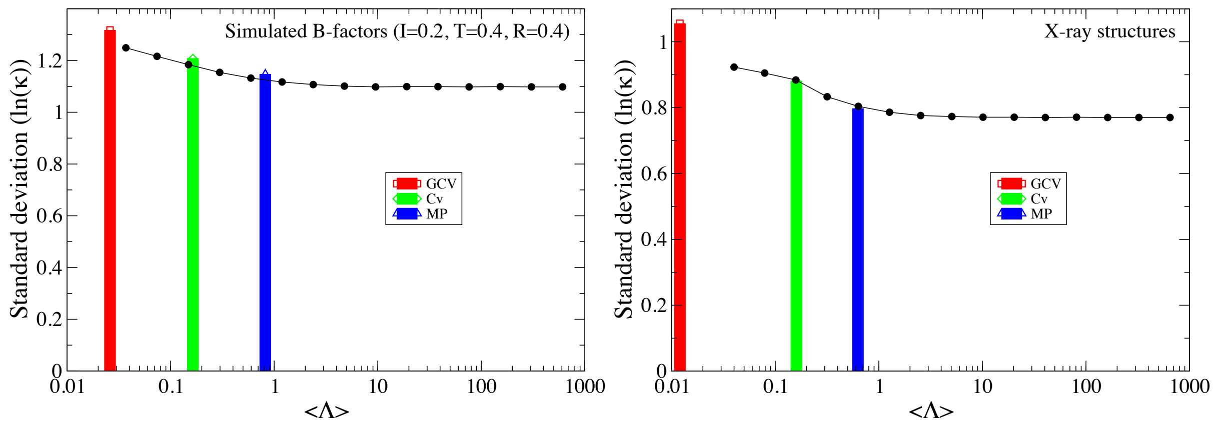


**Supplementary Figure S5: Standard deviation of the logarithm of the force constant versus the average ridge parameter.** Results are given for the simulated set with $I = 0.2$ and $T = R$ (left), and the X-ray dataset (right).
